# Supplementary material for: Anomalous Enhancement of the Electrocatalytic Hydrogen Evolution Reaction in AuPt Nanoclusters
Source: arXiv:2406.08580 ancillary file (2024-06-12)
Supplement: Supplementary file 1 [file SI_computational.pdf]

# Appendix 2: Supporting information with computational details

## Anomalous Enhancement of the Electrocatalytic Hydrogen Evolution Reaction in AuPt Nanoclusters

An accurate description of the energetics of AuPt nanoclusters (NCs) and their interaction with hydrogen can in principle be obtained within density functional theory (DFT). However, these calculations quickly become intractable as the number of atoms increases. To overcome this problem, we train a machine-learning potential (MLP) [1] from DFT data, which affords us the ability to perform millions of calculations for the NC sizes of interest in this work, with accuracy close to that of DFT but with affordable computational cost.

We train the AuPt:H MLP following the recipe presented in detail in Ref. [2]. Briefly, we generate DFT training data at the PBE level [3] with the VASP code [4, 5]. The training database contains basic crystal structures, dimers, trimers, liquids, surfaces, and NCs for AuPt. The incorporation of H-containing structures into the training database is done by iteratively training [6, 7] the MLP adding AuPt NPs of variable composition with also variable amounts of adsorbed hydrogen. Our MLP is of the Gaussian approximation potential (GAP) type [8], with two-body and smooth overlap of atomic positions (SOAP) descriptors [9, 10]. Fitting of the GAP is carried out with the QUIP/GAP code [11–13] and the different atomistic simulations reported here are performed with the TurboGAP code [14]. The Atomic Simulation Environment (ASE) is used for various atomistic structure analyses and manipulations [15]. The new GAP has been made freely available from the Zenodo repository [16].

We start by generating structural models of the AuPt NCs. According to the estimates from experiment, NCs containing circa 350 metal atoms are the most representative, and so we focus on this size range.

We follow the high-temperature simulated-annealing protocol that we have successfully used for Pt and Fe NPs [2, 17]. We initialize with a spherical NC with the target composition and run molecular dynamics (MD) at the annealing temperature. Here we systematically look for the optimal annealing temperature by searching above and below the estimated optimal annealing temperature $T_0$ of AuPt, which is calculated for $\mathrm{Pt}_{1-x}\mathrm{Au}_x$ from:

$$T_0(x) = 750x + 1150(1-x)\,\mathrm{K}, \tag{1}$$

where 1150 K is the optimal annealing temperature found for pure Pt NCs [2] and 750 K is that estimated for pure Au NCs extrapolating from the ratio of experimental melting temperatures of Au and Pt. To ensure the actual optimal temperature is not missed, we perform simulations at 5 % intervals between 90 % and 120 % of $T_0$. We explore values of $x \in [0, 1]$ at $\Delta x = 0.1$ intervals, and run 10 independent simulations for each composition, to avoid random bias due to the starting positions in the initial spherical structure. Therefore, the survey 11 compositions at 7 different annealing temperatures and 10 independent starting configurations per combination, resulting in 770 trajectories in total.

The annealing MD stage is carried out for 100 ps (with 4 fs time step), followed by a quench stage with linearly decreasing temperature profile down to 100 K over another 100 ps of MD, followed by a gradient-descent geometry optimization to the nearest local minimum of the potential energy surface. In the MD simulations the temperature is controlled with a Bussi thermostat [18] with time constant 100 fs.

In MCMC simulations, we sequentially add or remove hydrogens to reach the equilibrium

$$[\mathrm{NC{:}H}]^{(i)} + \mathrm{H}^* \rightleftharpoons [\mathrm{NC{:}H}]^{(i)} + \mathrm{H}^+(\mathrm{aq/vac}) + e_V^-, \tag{2}$$

where NC:H is a given NC with (some) adsorbed hydrogen on it, $\mathrm{H}^*$ is an additional adsorbed hydrogen, $\mathrm{H}^+$ is a free proton either in aqueous environment or vacuum, and $e_V^-$ is an electron at a given electrode potential $V$. The index $i$ indicates the current step in the MCMC sequence and the equilibrium is reached for $i \to \infty$, which will determine the amount of adsorbed hydrogen at equilibrium for a given $V$. We can rewrite this equilibrium relation in terms of potential energy:

$$E_{\mathrm{NC}} + E_{\mathrm{H}^*} \rightleftharpoons E_{\mathrm{NC}} + \underbrace{E_{\mathrm{H}^+} - eV}_{\mu_{\mathrm{H}}}, \tag{3}$$

where $e$ is now the elemental charge and we have simplified the notation for clarity. This form of the equation allows us to identify the equivalent chemical potential $\mu_{\mathrm{H}}$, which is what we actually tune in the MCMC simulation since we do not have an explicit electrode acting as electron reservoir. Equations (2) and (3) provide the intuitive means to understand the role of the chemical potential and its connection with the electrochemical problem: if the potential $V$ is increased, the potential energy of the free electron is lowered and the equilibrium "moves" to the right hand side, leading to hydrogen desorption. This is the same as lowering the chemical potential. Conversely, decreasing the potential $V$ leads to enhanced adsorption, and it is equivalent to increasing the chemical potential. Therefore, the chemical potential is proportional to the potential, with $-e$ (minus the elementary charge) being the proportionality constant. We also note that this approach does not explicitly account for kinetics.

The MCMC hydrogenation simulations progress in the following way. There is an equal probability of attempting addition or removal of a hydrogen atom to the NCs. After addition or removal, the whole structure is optimized and its energy computed. The addition/removal move is accepted or rejected according to the Metropolis criterion with appropriate prefactors. The probability $p$ to accept the move is:

$$p_{\mathrm{addition}} = \min\left\{1, \frac{M - N_{\mathrm{H}}}{N_{\mathrm{H}} + 1} \mathrm{e}^{\frac{-(E_i - (E_{i-1} + \mu_{\mathrm{H}}))}{k_{\mathrm{B}}T}}\right\}, \quad (4)$$

$$p_{\mathrm{removal}} = \min\left\{1, \frac{N_{\mathrm{H}}}{M + 1 - N_{\mathrm{H}}} \mathrm{e}^{\frac{-(E_i - (E_{i-1} - \mu_{\mathrm{H}}))}{k_{\mathrm{B}}T}}\right\}, \quad (5)$$

where $M$ is the total number of adsorption sites, which we estimate by combining all the existing top, bridge and hollow sites on the NC's surface. $N_{\mathrm{H}}$ is the number of currently adsorbed hydrogens. As expected, if all adsorption sites are occupied, $M - N_{\mathrm{H}} = 0$, and so the probability of addition is zero regardless of the outcome of the energy comparison. Likewise, if $N_{\mathrm{H}} = 0$ no hydrogens can be removed. The energy scale is provided by the $k_{\mathrm{B}}T$ term, which allows us to set a non-zero likelihood of acceptance for moves that increase the system's energy but are within the range of thermal activation. In our study we use $T = 300$ K. The approach is very similar to that given in Ref. [19], but we have corrected the prefactors. Correct prefactors are very important in our case because at the chemical potentials where the relevant adsorption/desorption processes are taking place the energy differences between structures before and after a MCMC move can be quite small.

We ran MCMC trajectories for all studied compositions between $\mu = -3$ eV and $\mu = 0$ eV. For each combination of initial structure and chemical potential we ran 10 different trajectories to account for random effects, for a total of 1760 trajectories. For each trajectory, we ran 2000 MCMC steps, and each structural optimization was allowed up to 1000 gradient-descent updates to achieve convergence. Therefore, we have performed of the order of one billion individual evaluations of the potential energy surface, a feat clearly infeasible at the DFT level of theory and only possible with the help of an MLP. All of our trajectories are freely available from Zenodo [20].


[1] V. L. Deringer, M. A. Caro, and G. Csányi, "Machine learning interatomic potentials as emerging tools for materials science," Adv. Mater. **31**, 1902765 (2019).

[2] J. Kloppenburg, H. Pártay, L. B .and Jónsson, and M. A. Caro, "A general-purpose machine learning pt interatomic potential for an accurate description of bulk, surfaces, and nanoparticles," J. Chem. Phys. **158**, 134704 (2023).

[3] J. P. Perdew, K. Burke, and M. Ernzerhof, "Generalized gradient approximation made simple," Phys. Rev. Lett. **77**, 3865 (1996).

[4] G. Kresse and J. Furthmüller, "Efficient iterative schemes for *ab initio* total-energy calculations using a plane-wave basis set," Phys. Rev. B **54**, 11169 (1996).

[5] G. Kresse and D. Joubert, "From ultrasoft pseudopotentials to the projector augmented-wave method," Phys. Rev. B **59**, 1758 (1999).

[6] V. L. Deringer and G. Csányi, "Machine learning based interatomic potential for amorphous carbon," Phys. Rev. B **95**, 094203 (2017).

[7] T. Zarrouk, R. Ibragimova, A. P. Bartók, and M. A. Caro, "Experiment-driven atomistic materials modeling: A case study combining x-ray photoelectron spectroscopy and machine learning potentials to infer the structure of oxygen-rich amorphous carbon," J. Am. Chem. Soc. **(in press)** (2024).

[8] A. P. Bartók, M. C. Payne, R. Kondor, and G. Csányi, "Gaussian approximation potentials: The accuracy of quantum mechanics, without the electrons," Phys. Rev. Lett. **104**, 136403 (2010).

[9] A. P. Bartók, R. Kondor, and G. Csányi, "On representing chemical environments," Phys. Rev. B **87**, 184115 (2013).

[10] M. A. Caro, "Optimizing many-body atomic descriptors for enhanced computational performance of machine learning based interatomic potentials," Phys. Rev. B **100**, 024112 (2019).

[11] G. Csányi, S. Winfield, J. R. Kermode, A. De Vita, A. Comisso, N. Bernstein, and M. C. Payne, "Expressive programming for computational physics in Fortran 95+," IoP Comput. Phys. Newsletter , Spring 2007 (2007).

[12] https://libatoms.github.io.

[13] S. Klawohn, J. P. Darby, J. R. Kermode, G. Csányi, M. A. Caro, and A. P. Bartók, "Gaussian approximation potentials: theory, software implementation and application examples," J. Chem. Phys. **159**, 174108 (2023).

[14] M. A. Caro *et al.*, "TurboGAP: Data-driven atomistic simulations," `http://turbogap.fi`, accessed: 2023-02-17.

[15] A. H. Larsen, J. J. Mortensen, J. Blomqvist, I. E. Castelli, R. Christensen, M. Dulak, J. Friis, M. N. Groves, B. Hammer, C. Hargus, E. D. Hermes, P. C. Jennings, P. B. Jensen, J. Kermode, J. R. Kitchin, E. L. Kolsbjerg, J. Kubal, K. Kaasbjerg, S. Lysgaard, J. B. Maronsson, T. Maxson, T. Olsen, L. Pastewka, A. Peterson, C. Rostgaard, J. Schiøtz, O. Schütt, M. Strange, K. S. Thygesen, T. Vegge, L. Vilhelmsen, M. Walter, Z. Zeng, and K. W. Jacobsen, "The Atomic Simulation Environment – A Python library for working with atoms," J. Phys.: Condens. Matter **29**, 273002 (2017).

[16] J. Kloppenburg and M. A. Caro, "GAP interatomic potential for PtAu:H nanoparticle simulation," Zenodo (2024), DOI:10.5281/zenodo.11184038.

[17] R. Jana and M. A. Caro, "Searching for iron nanoparticles with a general-purpose Gaussian approximation potential," arXiv:2302.13722 (2023).

[18] G. Bussi, D. Donadio, and M. Parrinello, "Canonical sampling through velocity rescaling," J. Chem. Phys. **126**, 014101 (2007).

[19] V. L. Deringer, M. A. Caro, R. Jana, A. Aarva, S. R.

Elliott, T. Laurila, G. Csányi, and L. Pastewka, "Computational surface chemistry of tetrahedral amorphous carbon by combining machine learning and DFT," Chem. Mater. **30**, 7438 (2018).

[20] J. Kloppenburg and M. A. Caro, "Structural database of small PtAu and hydrogenated PtAu nanoparticles," Zenodo (2024), DOI:10.5281/zenodo.11185692.
