# Supplementary material for: Anomalous Enhancement of the Electrocatalytic Hydrogen Evolution Reaction in AuPt Nanoclusters
Source: arXiv:2406.08580 ancillary file (2024-06-12)
Supplement: Supplementary file 2 [file SI_experimental.pdf]

Appendix 1: Supporting information with experimental details

# Anomalous Enhancement of the Electrocatalytic Hydrogen Evolution Reaction in AuPt Nanoclusters

## Experimental section

*Synthesis of carbon nanotubes (CNTs):*

The synthesis method used in this study is based on previously reported work.[1] Initially, ferrocene (2 wt.%) and thiophene were mixed in a molar ratio of Fe/S = 2.5 and dissolved in 5 mL of toluene. The solution was sonicated for 1 minute and then loaded into a 10 mL glass syringe. Using a syringe pump (NE-1000 series, New York) and a Teflon piston tip (Innovative Labor Systeme, Germany), the mixture was injected at a rate of 0.6 mL/h into a floating catalyst chemical vapor deposition system.[2] The solution was evaporated in a heated line at 130 °C, and the vaporized precursor was carried by a gas mixture of $H_2$ (1.5 standard liters per minute, slm) and $N_2$ (10 slm). The reaction temperature was set to 1180 °C. CNTs were collected at the furnace outlet onto a membrane filter, forming a film that could be transferred to the target substrate for characterization.

The obtained CNT was processed with sulfuric acid for 24 h, and then washed with DI water for several times, and finally stored at room temperature for further use.

*Synthesis of Au-CNT, $Au_{0.8}Pt_{0.2}$-CNT, $Au_{0.6}Pt_{0.4}$-CNT, $Au_{0.4}Pt_{0.6}$-CNT, $Au_{0.2}Pt_{0.8}$-CNT, Pt-CNT films:*

The $H_2SO_4$-processed CNT films were put into 2mL $Au_xPt_{1-x}$ NCs dispersion for 20h.

*Synthesis of Au-CNT-A,* $Au_{0.8}Pt_{0.2}$*-CNT-A,* $Au_{0.6}Pt_{0.4}$*-CNT-A,* $Au_{0.2}Pt_{0.8}$*-CNT-A, Pt-CNT-A films:*

The methods for synthesis of $Au_xPt_{1-x}$-CNT-A films are similar with $Au_{0.4}Pt_{0.6}$-CNT-A film, except using the precursors of $Au_xPt_{1-x}$-CNT film with different Au/Pt feed ratio, respectively.

*Synthesis of* $Au_{0.4}Pt_{0.6}$*-A:*

The $Au_{0.4}Pt_{0.6}$ powders by freezing drying was put into the tube furnace at 300 ℃ for 30 min annealing under $N_2$ protection. After annealing, the $Au_{0.4}Pt_{0.6}$-A was prepared.

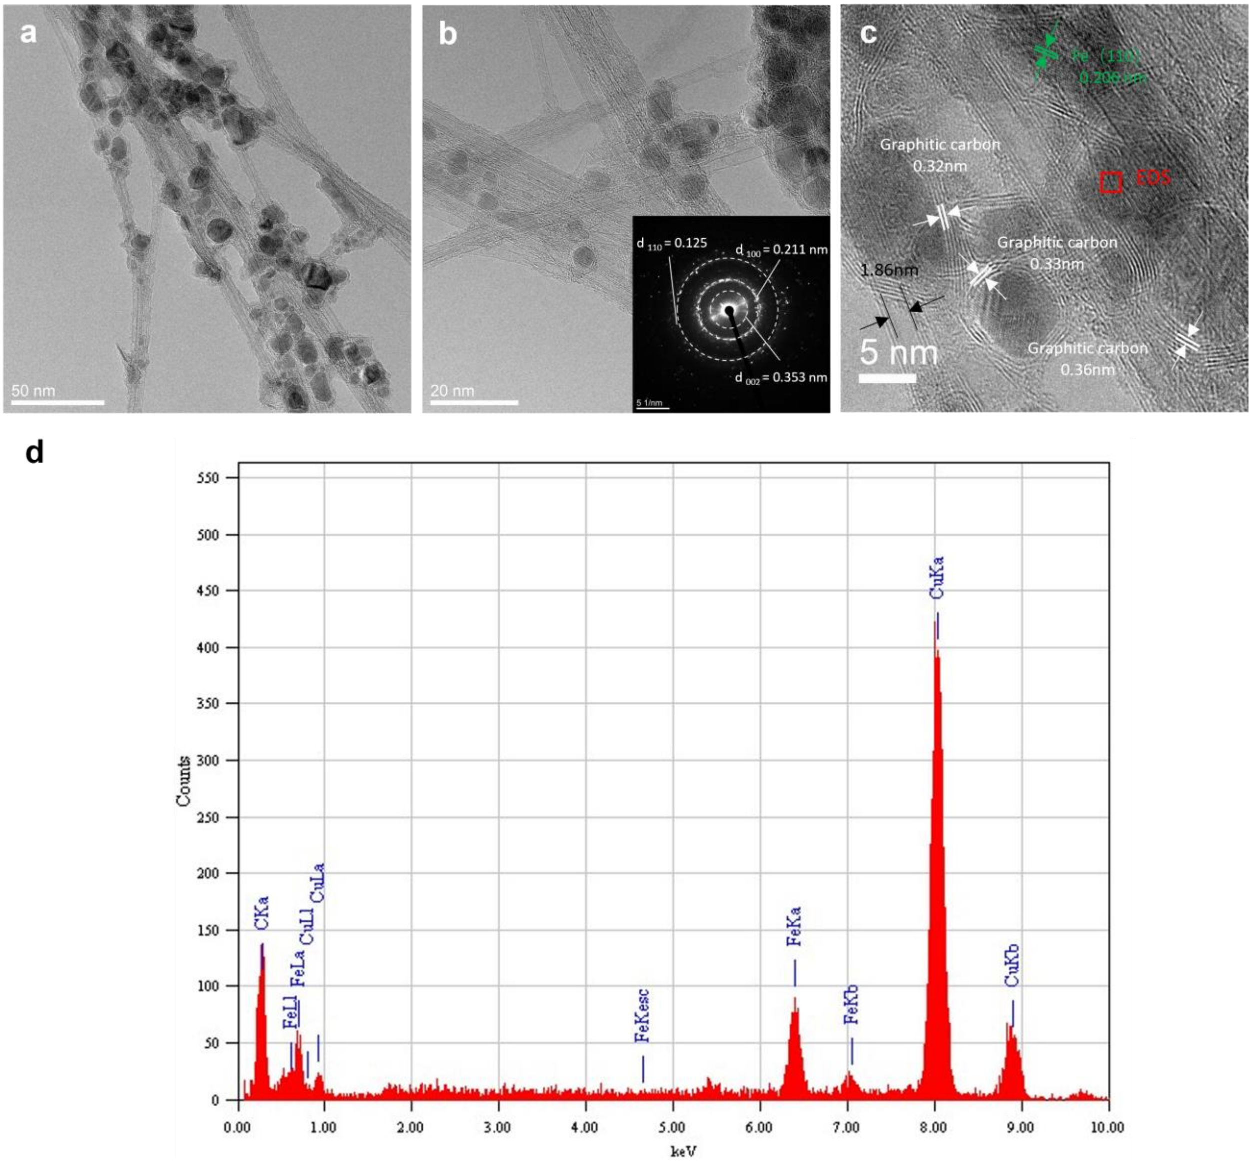


Figure S1. TEM images of pristine CNT. EDS confirms the existence of Fe. (Red fame in c): the position of EDS area analysis)

High-resolution TEM (HRTEM) and energy dispersive spectrometry (EDS) elemental analysis indicate that the pristine CNTs are grown by nucleation on Fe nanoparticles, formed from the decomposition of the ferrocene precursor. The selected area electron diffraction (SAED) pattern confirms the presence of (110), (100) and (002) of the graphitic carbon.[3]

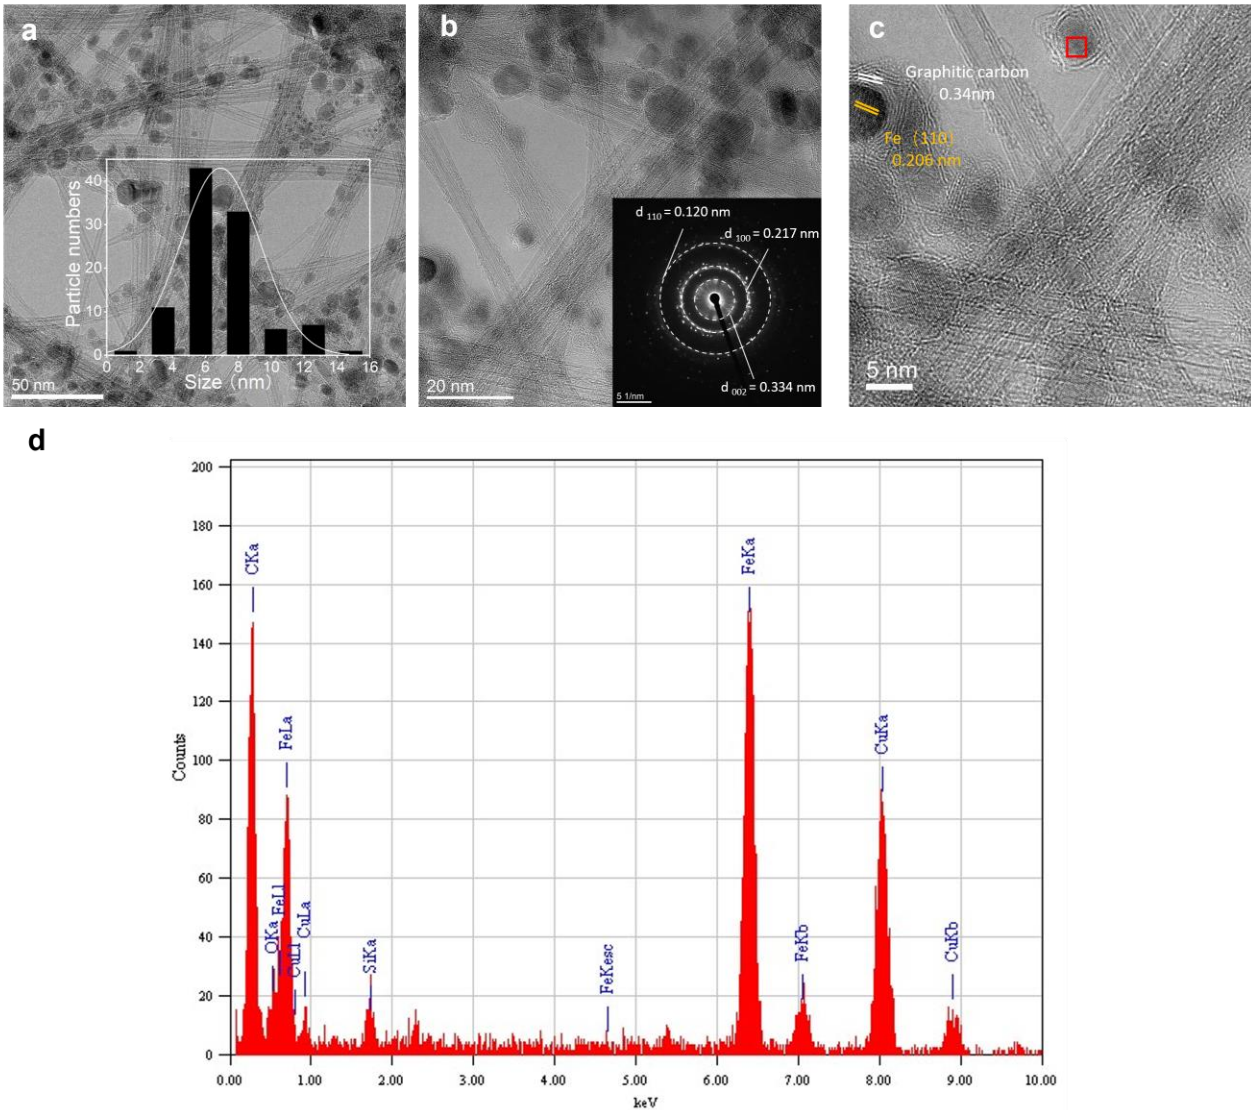


Figure S2. a-b) TEM images (Polydispersity index = 0.11) and c-d) EDS analysis of sulfated CNT. (Red fame in c): the position of EDS area analysis)

The EDS elemental analysis of the selected particles confirmed the existence of graphitic carbon and polydisperse Fe with approximate diameters of ~2-15 nm.

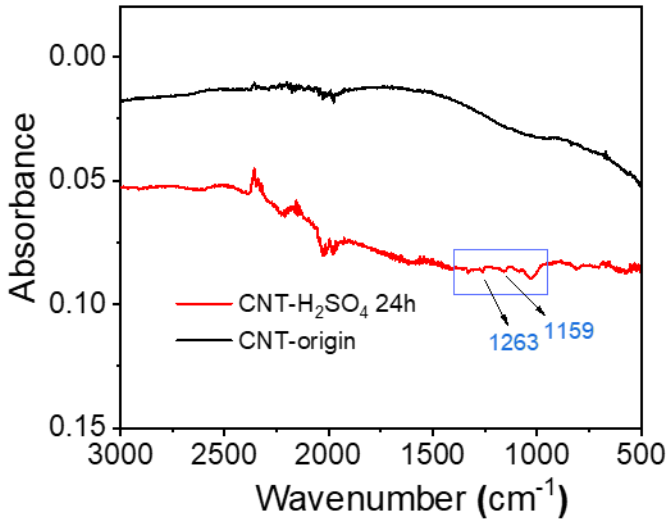


Figure S3. FTIR of the sulfated CNT and pristine CNT.

Moreover, by comparing the FTIR spectra (Figure S3) of the processed CNT with the pristine CNT, the peaks of O=S=O were observed at 1159 $cm^{-1}$ and 1263 $cm^{-1}$ after processing with $H_2SO_4$ because of the symmetric and asymmetric stretching vibrations of S=O groups, hinting the doping of $-OSO_3H$ groups on CNTs.[4]

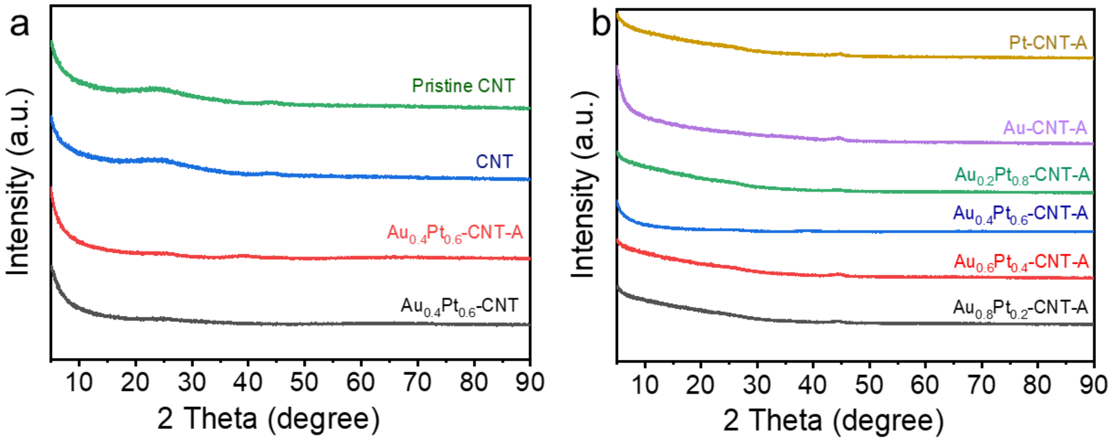


Figure S4. XRD of $Au_{0.4}Pt_{0.6}$-CNT-A and compared samples.

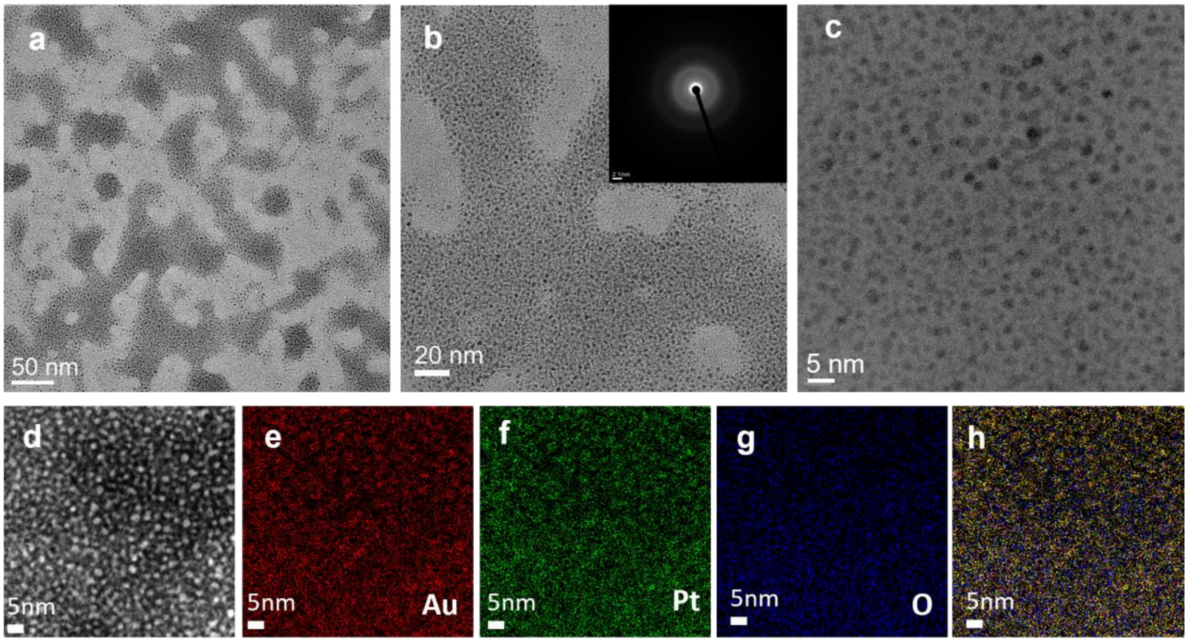


Figure S5. a-c) TEM images (inset of b) SAED patterns of $Au_{0.4}Pt_{0.6}$ NCs). d-h) EDS mapping of $Au_{0.4}Pt_{0.6}$ NCs (h: overlay of Au, Pt, and O).

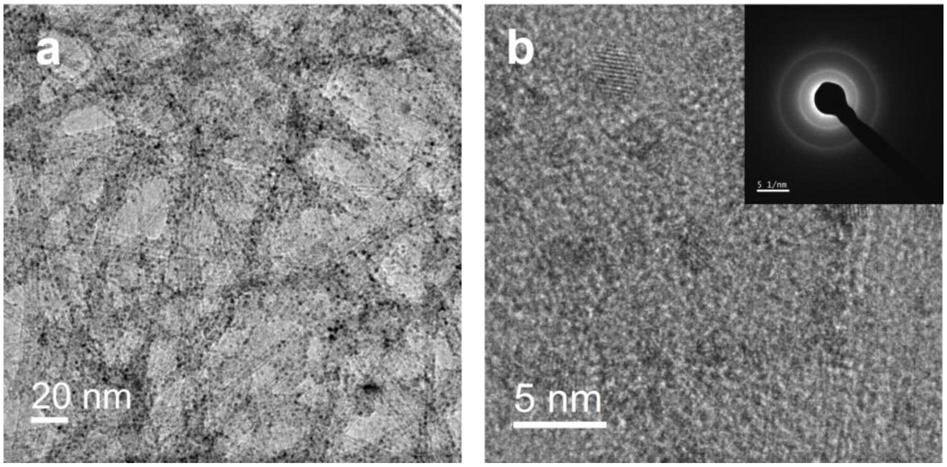


Figure S6. TEM images of $Au_{0.4}Pt_{0.6}$-CNT.

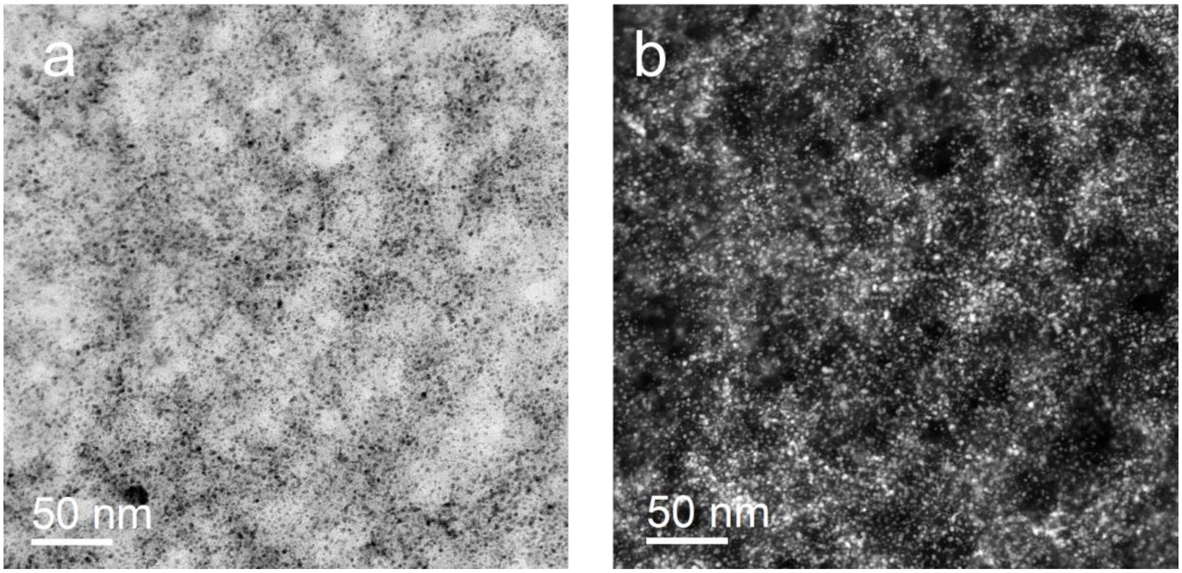


Figure S7. a-b) TEM images on bright-field (BF) and dark-field (DF) of $Au_{0.4}Pt_{0.6}$-CNT-A.

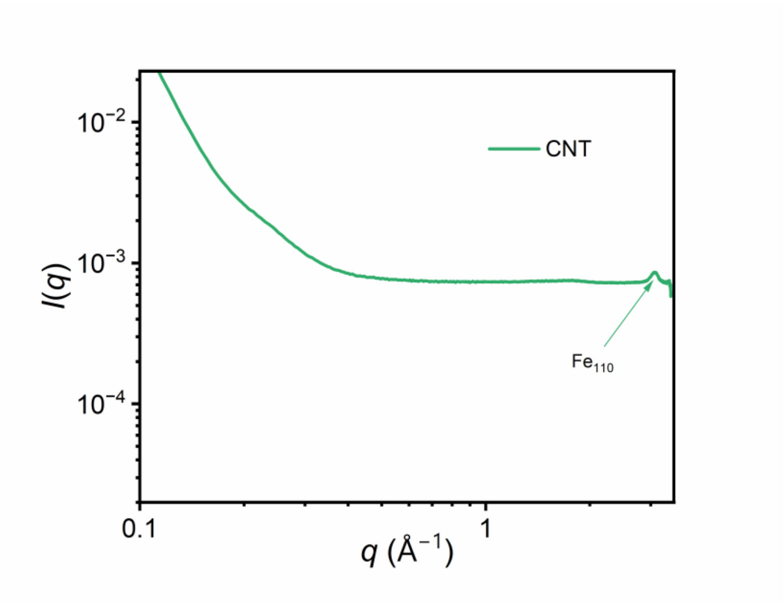


Figure S8. WAXS of CNT film.

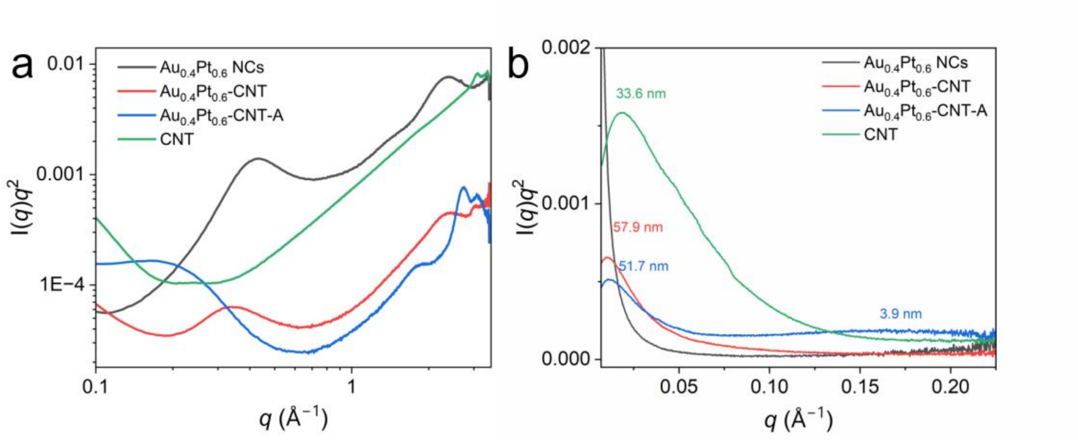


Figure S9. WAXS and SAXS result of $Au_{0.4}Pt_{0.6}$-CNT-A film, $Au_{0.4}Pt_{0.6}$-CNT film, CNT film and $Au_{0.4}Pt_{0.6}$ NCs powder.

Table S1. Average Diameter, ⟨d⟩, Resulting from WAXS and SAXS Data Analysis

| | q (Å$^{-1}$) | Average diameter, ⟨d⟩ (nm) | Note |
|---|---|---|---|
| $Au_{0.4}Pt_{0.6}$ NCs | 0.433 | 1.45 | Cluster-cluster |
| | 2.21 | 0.280 | Atom-atom |
| $Au_{0.4}Pt_{0.6}$ NCs-CNT | 0.343 | 1.83 | Cluster-cluster |
| | 2.21 | 0.280 | Atom-atom |
| $Au_{0.4}Pt_{0.6}$ NCs-CNT-A (annealing) | 0.173 | 3.63 | Cluster-cluster |
| | 1.75 | 0.358 | Atom-atom |
| | 2.69 | 0.233 | Au-Pt (111) |
| | 3.08 | 0.203 | Au-Pt (200) |
| CNT | 3.06 | 0.206 | Fe (110) |

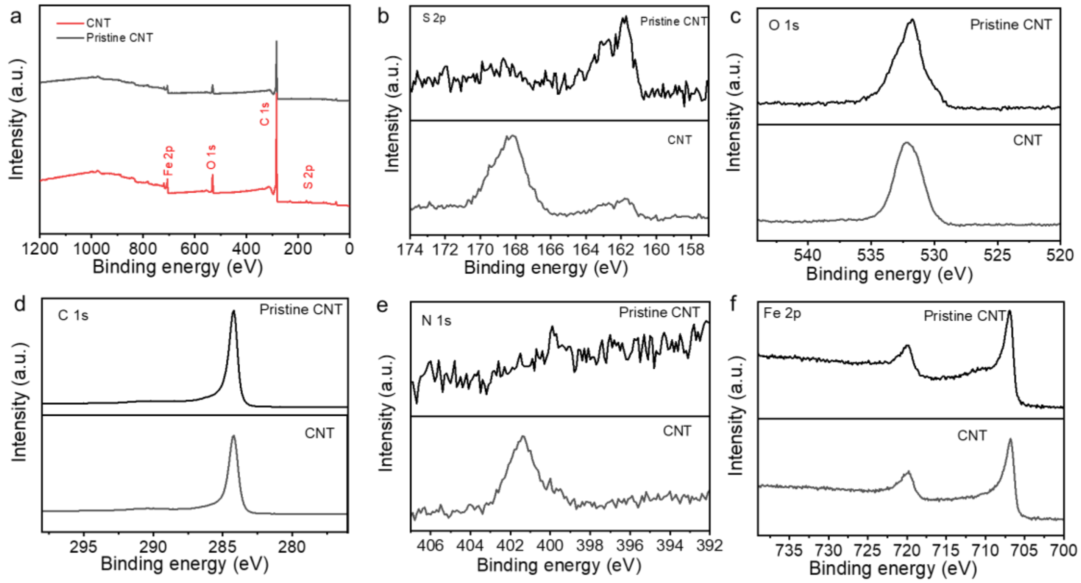


Figure S10. XPS of CNT and pristine CNT (red line: CNT processed by $H_2SO_4$).

Besides, compared with the survey spectrum of pristine CNT (Figure S16 and Table S2), the processed CNT has a high signal of S-O for S $2p_{3/2}$ peak, confirming the formation of -$OSO_3$ after sulfuric acid treatment, which is consistent with the FTIR results. Furthermore, the XPS spectra of the CNT also exhibit the existence of Fe in both pristine CNT and processed CNT, which is in line with TEM results.

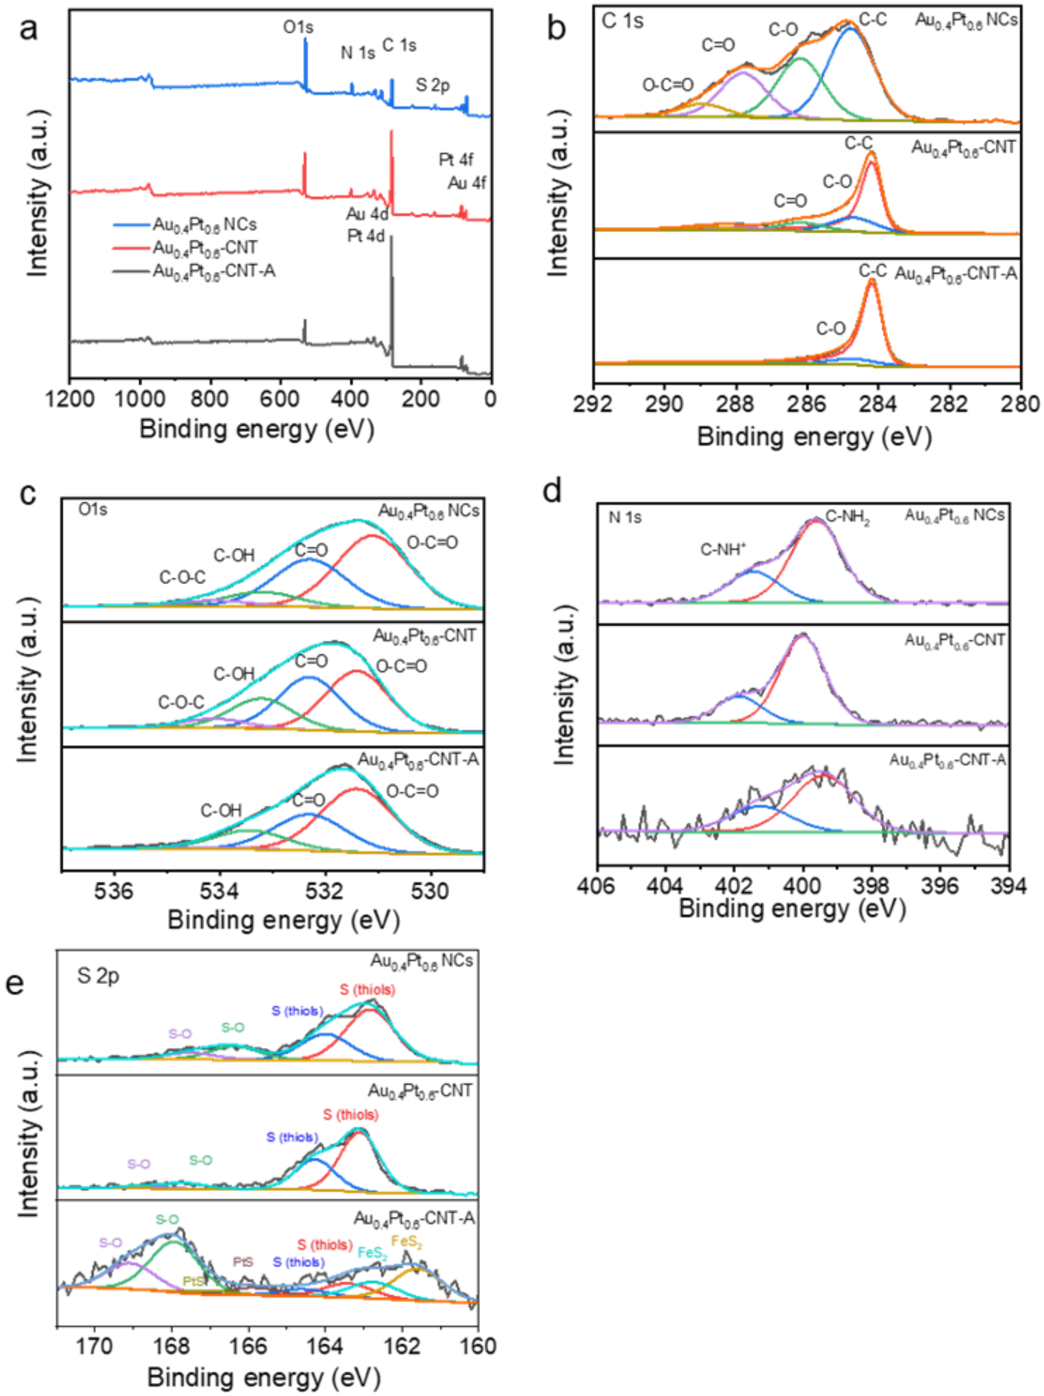


Figure S11. a) XPS survey, b) C1s, c) O1s and d) N1s, e) S2p spectra for $Au_{0.4}Pt_{0.6}$ NCs powder, $Au_{0.4}Pt_{0.6}$-CNT film, and $Au_{0.4}Pt_{0.6}$-CNT-A film. (All the samples are corrected with respect to carbon, for powder: use 248.8 eV; for films: use 248.2 eV)

Table S2. Relative concentrations of elements in the $Au_{0.4}Pt_{0.6}$ NCs, $Au_{0.4}Pt_{0.6}$-CNT, $Au_{0.4}Pt_{0.6}$-CNT-A.

| Sample | C 1s % | O 1s % | N 1s % | S 2p % | Au 4f % | Pt 4f % | Fe 2p % |
|---|---|---|---|---|---|---|---|
| $Au_{0.4}Pt_{0.6}$ NCs | 54.97 | 26.57 | 9.83 | 4.96 | 0.79 | 2.89 | 0.00 |
| $Au_{0.4}Pt_{0.6}$-CNT | 77.65 | 13.66 | 4.49 | 2.19 | 1.06 | 0.79 | 0.15 |
| $Au_{0.4}Pt_{0.6}$-CNT-A | 91.09 | 5.79 | 0.60 | 0.79 | 0.47 | 0.27 | 0.98 |

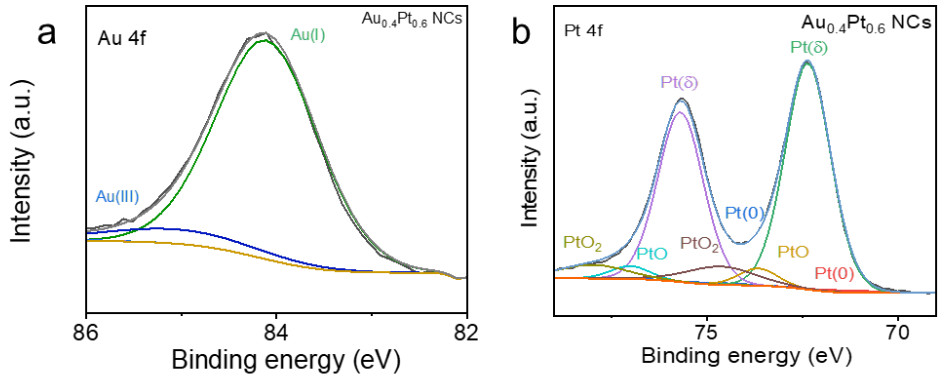


Figure S12. XPS of (a) Au 4f and (b) Pt 4f of $Au_{0.4}Pt_{0.6}$ NCs.

As shown in the reported work, the Au $4f_{7/2}$ of Au nanoclusters at 84.3 eV can be attributed to Au(I).[5] In addition, the Au $4f_{7/2}$ shape of AuPt NCs would shift to lower binding energy, compared with pure Au NCs according to the reported work.[6] Therefore, it is worth believing that the dominant peak of at 84.1 eV in $Au_{0.4}Pt_{0.6}$ NCs can be attributed to Au (I).

Table S3. $Au_{4f}$ and $Pt_{4f}$ spectra peak positions, Full-Width Half-Maxima of $Au_{0.4}Pt_{0.6}$ NCs, $Au_{0.4}Pt_{0.6}$ NCs-CNT and $Au_{0.4}Pt_{0.6}$ NCs-CNT-A.

| | Au4f$_{7/2}$ | | | | | | Pt4f$_{7/2}$ | | | | | | | |
|---|---|---|---|---|---|---|---|---|---|---|---|---|---|---|
| | Au(0) | | Au(I) | | Au(III) | | Pt(0) | | Pt(δ) | | Pt(II) | | Pt(IV) | |
| | Position (eV) | Fwhm (eV) | Position (eV) | Fwhm (eV) | Position (eV) | Fwhm (eV) | Position (eV) | Fwhm (eV) | Position (eV) | Fwhm (eV) | Position (eV) | Fwhm (eV) | Position (eV) | Fwhm (eV) |
| $Au_{0.4}Pt_{0.6}$ NCs | - | - | 84.10 | 1.26 | 85.04 | 1.89 | 71.16 | 1.80 | 72.36 | 1.40 | 73.66 | 1.20 | 74.44 | 2.11 |
| $Au_{0.4}Pt_{0.6}$ NCs-CNT | - | - | 84.49 | 1.03 | 85.43 | 1.55 | 71.54 | 1.15 | 72.74 | 1.15 | 74.03 | 1.15 | 75.04 | 1.15 |
| $Au_{0.4}Pt_{0.6}$ NCs-CNT-A | 83.68 | 0.88 | 84.62 | 0.88 | - | - | 70.89 | 1.26 | 72.08 | 1.26 | 73.38 | 1.26 | 74.38 | 1.26 |

The peaks positions of Au4f and Pt4f XPS deconvolution for $Au_{0.4}Pt_{0.6}$ NCs, $Au_{0.4}Pt_{0.6}$-CNT, $Au_{0.4}Pt_{0.6}$-CNT-A was as shown in Figure 1g, S12 and Table S3.

Table S4. S2p spectra peak positions of $Au_{0.4}Pt_{0.6}$ NCs, $Au_{0.4}Pt_{0.6}$ NCs-CNT and $Au_{0.4}Pt_{0.6}$ NCs-CNT-A.

| Sample | S (AuPt-S) | | S ($FeS_2$) | | S (S-O) | | S (S2^2-) | |
|---|---|---|---|---|---|---|---|---|
| | 2p$_{1/2}$(eV) | 2p$_{3/2}$ (eV) | 2p$_{1/2}$ (eV) | 2p$_{3/2}$ (eV) | 2p$_{1/2}$ (eV) | 2p$_{3/2}$ (eV) | 2p$_{1/2}$ (eV) | 2p$_{3/2}$ (eV) |
| $Au_{0.4}Pt_{0.6}$ NCs | - | - | - | - | 167.52 | 166.37 | 163.84 | 162.69 |
| $Au_{0.4}Pt_{0.6}$-CNT | - | - | - | - | 168.83 | 167.68 | 164.26 | 163.10 |
| $Au_{0.4}Pt_{0.6}$-CNT-A | 167 | 165.83 | 162.73 | 161.85 | 169.07 | 167.91 | 164.57 | 163.4 |

Table S5. Relative amounts of the different components of sulfur, as compared to the total intensity of sulfur in the samples.

| Sample | S (AuPt-S) % | S ($FeS_2$) % | S (S-O) % | S (S2^2-) % |
|---|---|---|---|---|
| $Au_{0.4}Pt_{0.6}$ NCs | - | - | 19.95 | 80.05 |
| $Au_{0.4}Pt_{0.6}$-CNT | - | - | 7.86 | 92.14 |
| $Au_{0.4}Pt_{0.6}$-CNT -A | 7.45 | 30.74 | 48.42 | 13.39 |

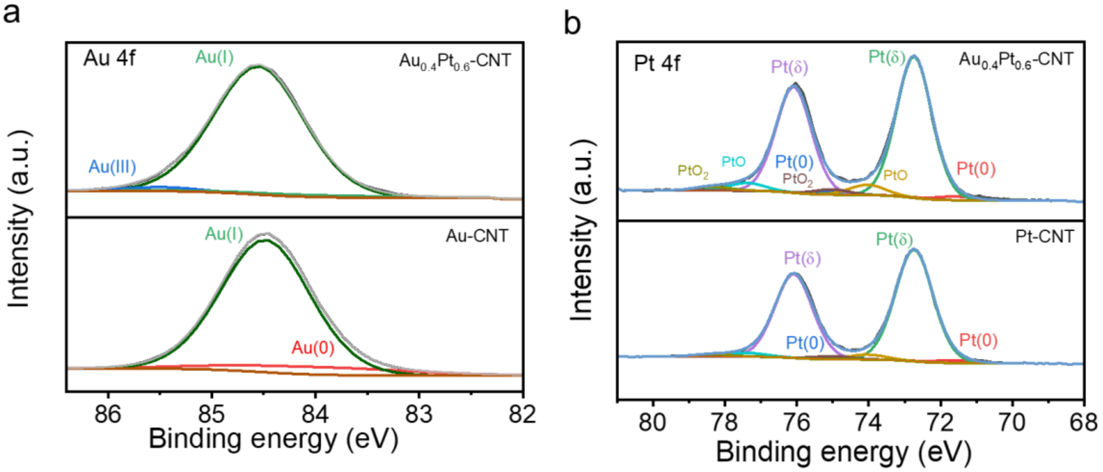


Figure S13. XPS of (a) Au 4f of $Au_{0.4}Pt_{0.6}$-CNT and Au-CNT, and (b) Pt 4f of $Au_{0.4}Pt_{0.6}$-CNT and Pt-CNT before annealing.

The Au(I) at 84.5 eV of Au $4f_{7/2}$ spectrum in the grafted $Au_{0.4}Pt_{0.6}$-CNT (Figure S13a) is identical to the Au(I) in Au-CNT; Pt(δ+) at Pt-CNT (Figure S13b) shows similar peak position.

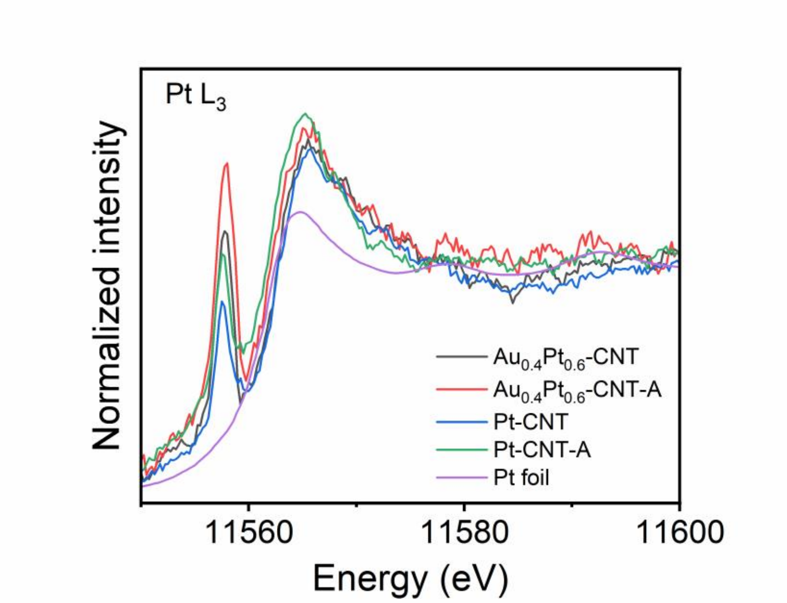


Figure S14. Normalized X-ray absorption near-edge structure (XANES) spectra at Pt $L_3$-edge of $Au_{0.4}Pt_{0.6}$-CNT-A and $Au_{0.4}Pt_{0.6}$-CNT, Pt-CNT-A, Pt-CNT and Pt foil.

The 'pre-edge' peak is a very strong monochromator glitch that happens to lie at this energy, ~11558 eV, and is not fully normalized out. The white line is quite higher for the CNT samples than for the foil, which means additional empty Pt $d_{5/2}$ states close to the Fermi level, i.e. somewhat oxidized state.

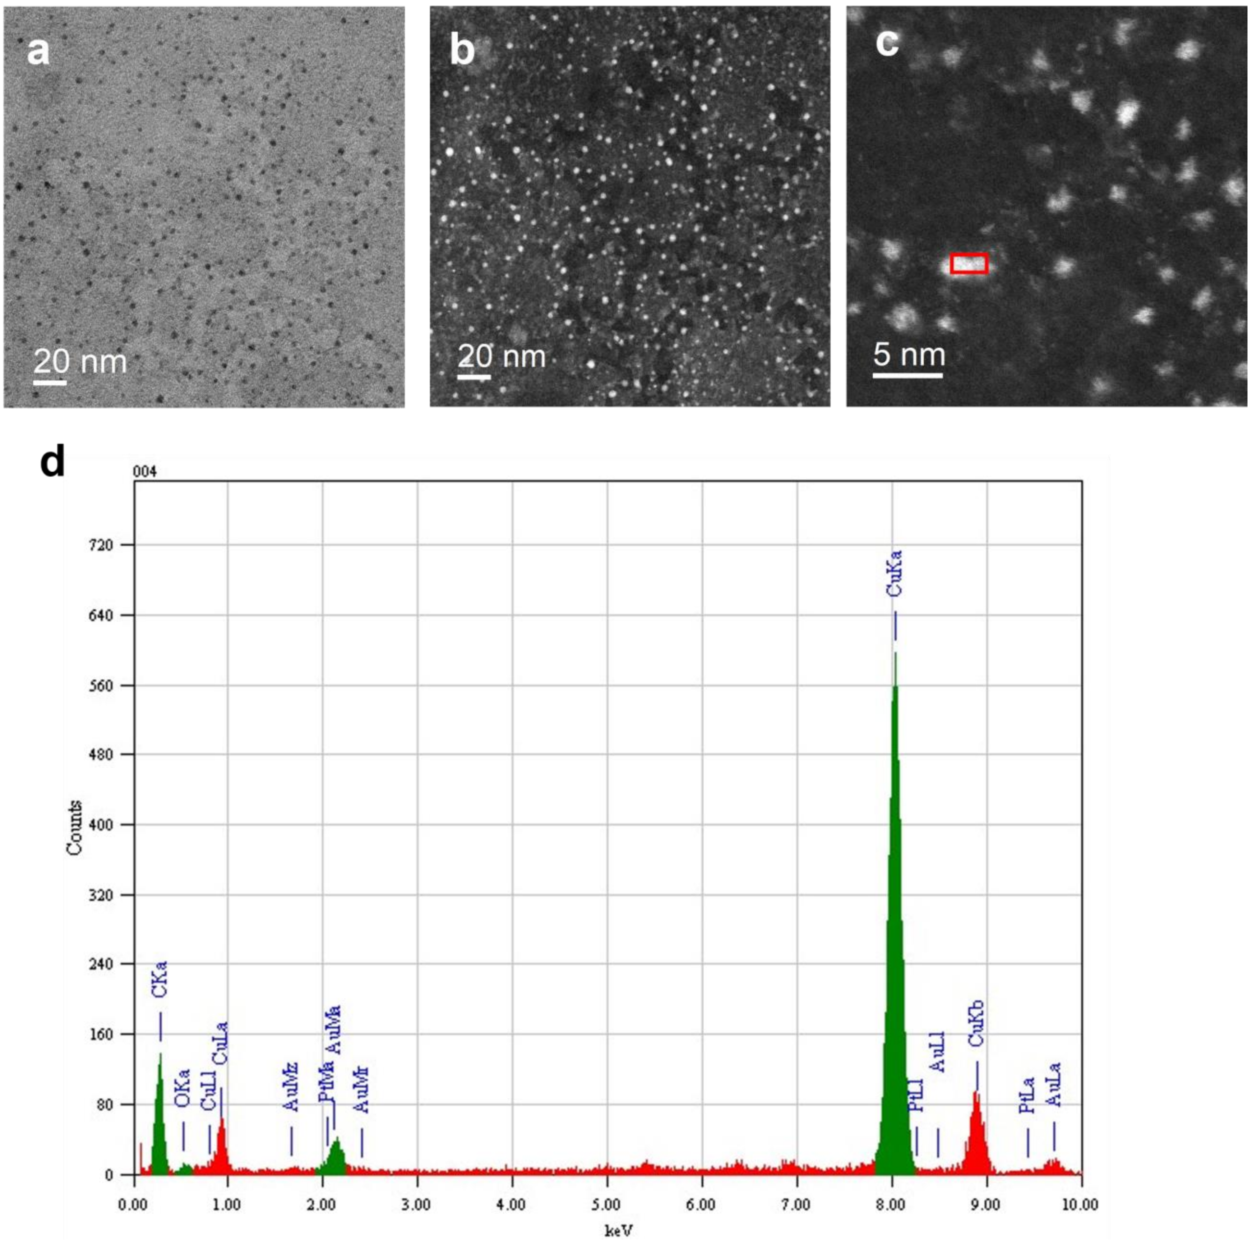


Figure S15. TEM images of $Au_{0.8}Pt_{0.2}$ NCs.

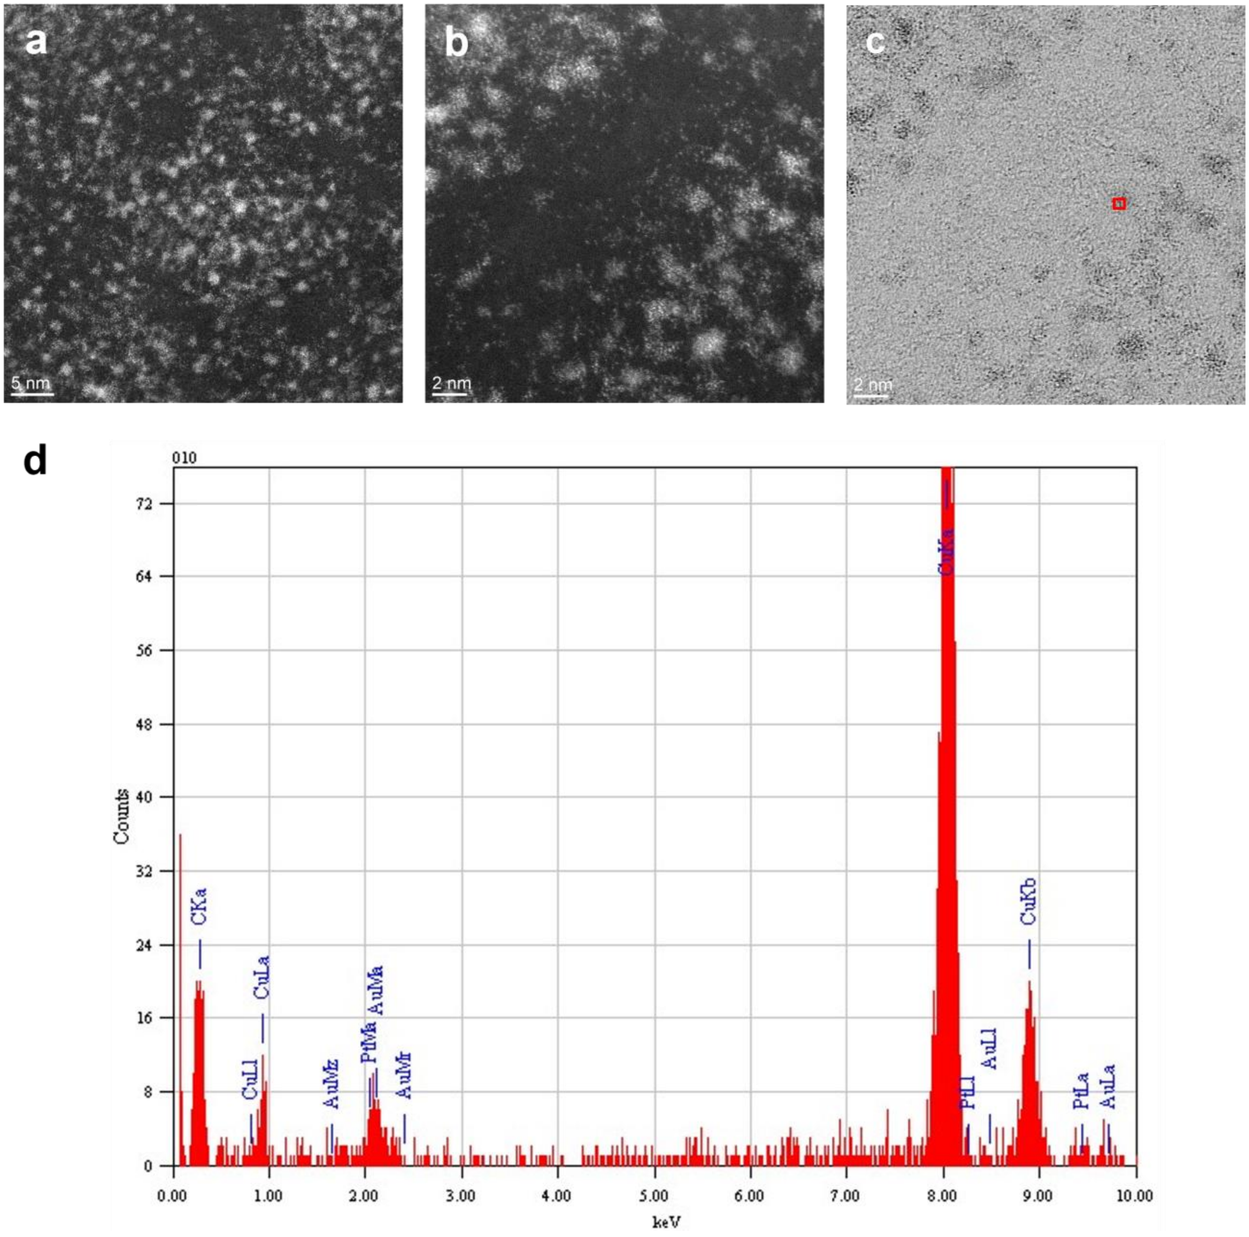


Figure S16. TEM images of $Au_{0.2}Pt_{0.8}$ NCs.

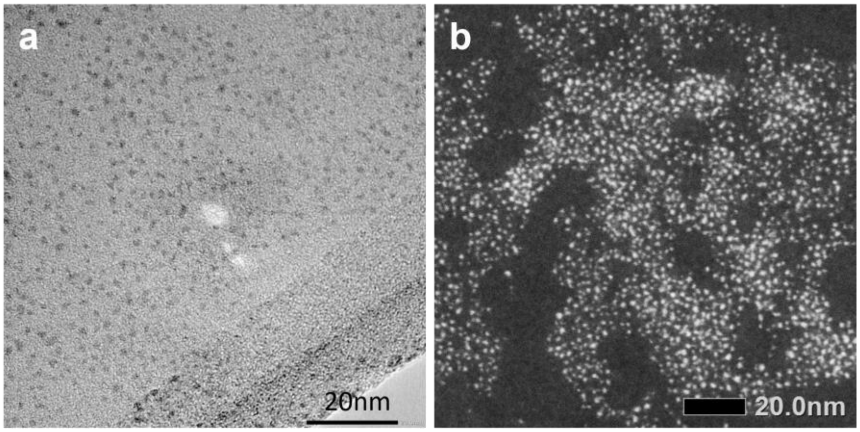


Figure S17. TEM images of Pt NCs.

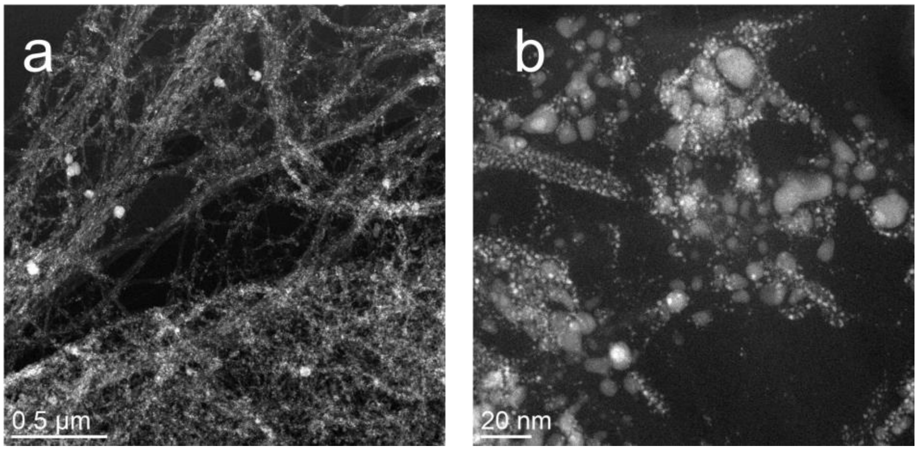


Figure S18. TEM images of Au-CNT.

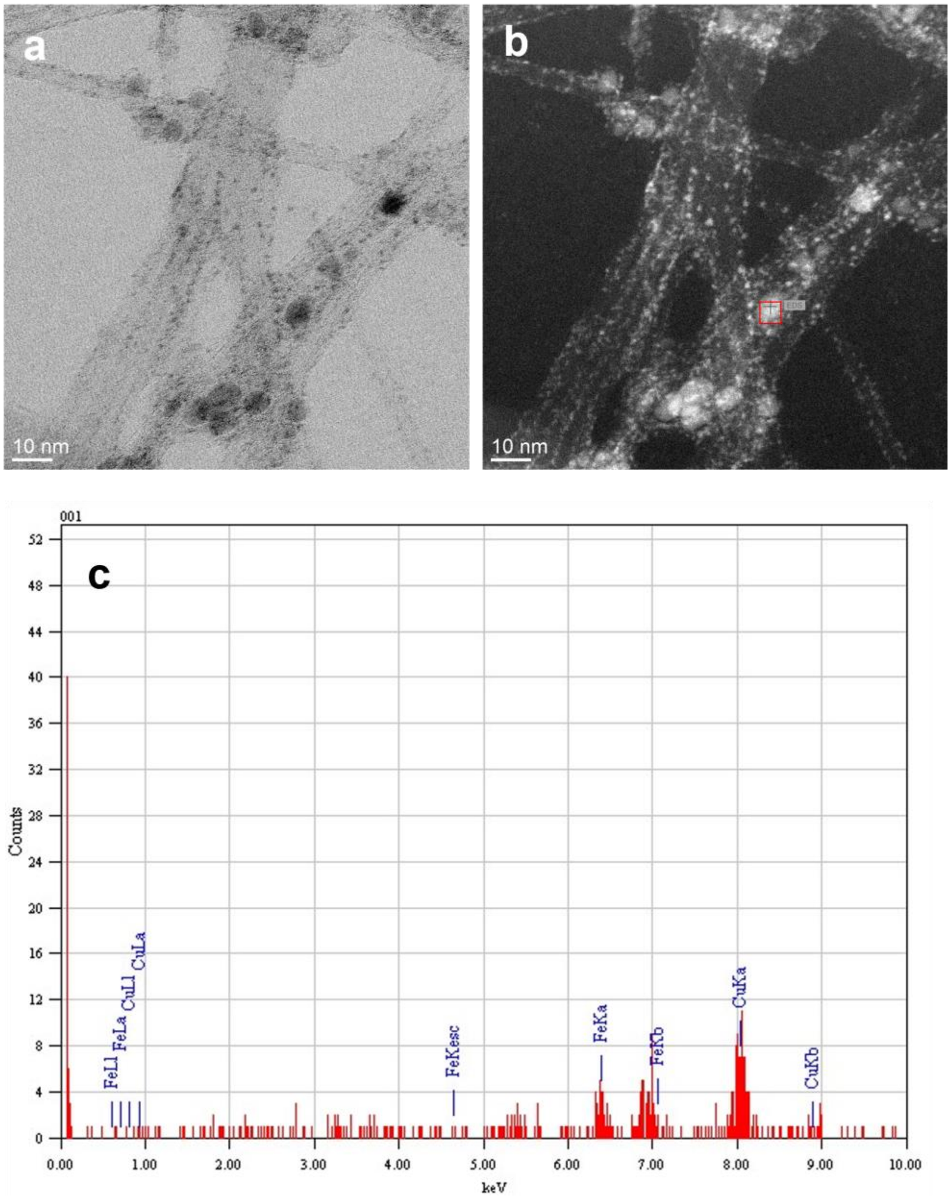


Figure S19. TEM images of $Au_{0.2}Pt_{0.8}$-CNT on a) BF and b) DF, and c) corresponding EDS analysis to the marked area (Fe particles).

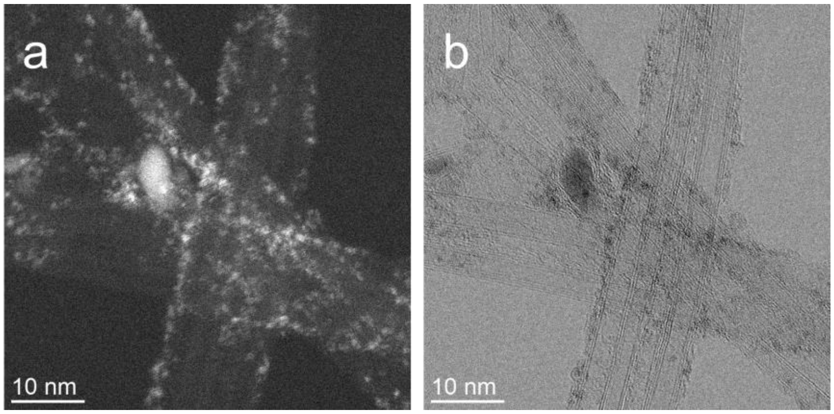


Figure S20. TEM images of Pt-CNT on DF and BF.

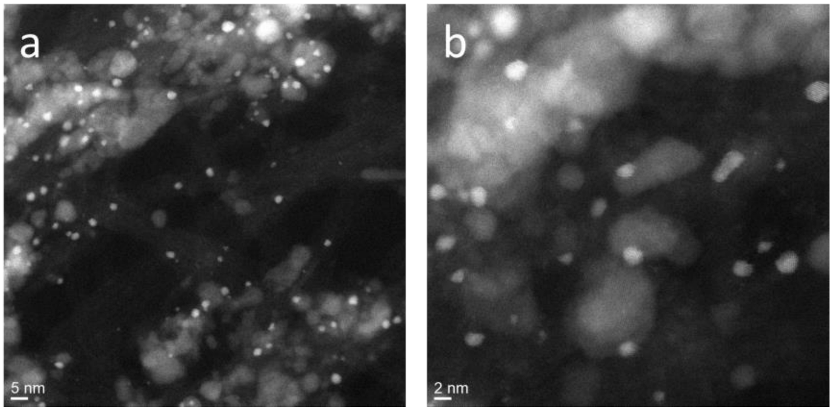


Figure S21. a-b) TEM images of Au-CNT-A on DF.

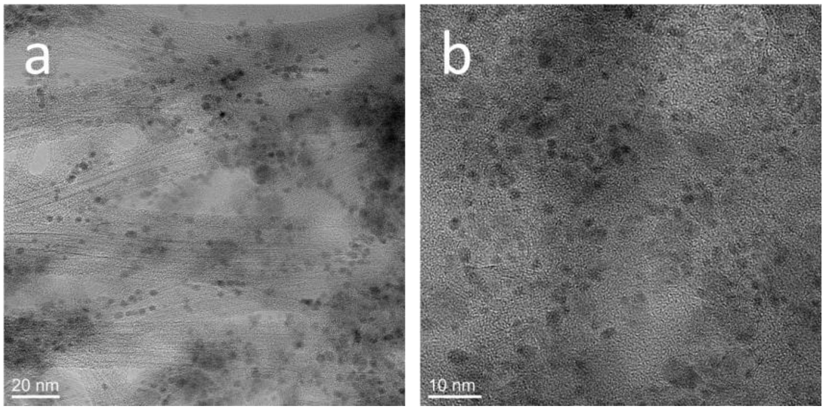


Figure S22. TEM images of Pt-CNT-A.

Table S6. ICP-OES result of $Au_{0.4}Pt_{0.6}$ -CNT-A and compared samples.

| | Au (ug /cm$^2$) | Pt (ug /cm2) | AuPt (ug /cm$^2$) | Au/Pt by weight | Au/Pt by atoms |
|---|---|---|---|---|---|
| $Au_{0.8}Pt_{0.2}$ -CNT-A | 9.54 | 7.20 | 16.74 | 1.32 | 1.31 |
| $Au_{0.6}Pt_{0.4}$ -CNT-A | 9.00 | 4.22 | 13.22 | 2.14 | 2.11 |
| $Au_{0.4}Pt_{0.6}$ -CNT-A | 5.75 | 10.94 | 16.69 | 0.56 | 0.52 |
| $Au_{0.2}Pt_{0.8}$ -CNT-A | 2.16 | 12.80 | 14.96 | 0.170 | 0.167 |
| Au -CNT-A | 51.88 | -- | 51.88 | -- | -- |
| Pt -CNT-A | -- | 12.55 | 12.55 | -- | -- |

The $Au_{0.8}Pt_{0.2}$-CNT-A, $Au_{0.6}Pt_{0.4}$-CNT-A, $Au_{0.4}Pt_{0.6}$-CNT-A, $Au_{0.2}Pt_{0.8}$-CNT-A, Au-CNT-A, Pt-CNT-A has a AuPt loading of 16.74, 13.22, 16.69, 14.96, 51.88 and 12.55 μg/cm$^2$, respectively.

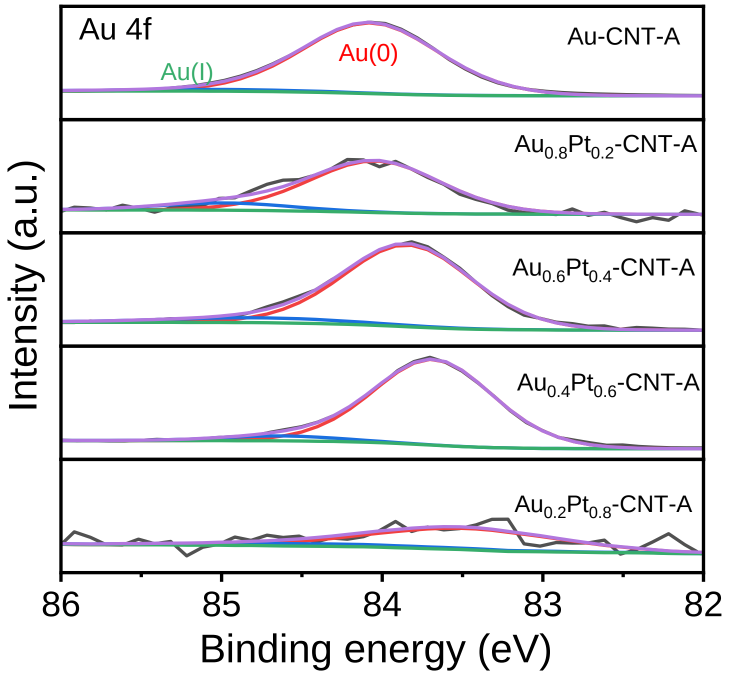


Figure S23. Au4f spectra of AuPt-CNT-A with different ratio of Au/Pt.

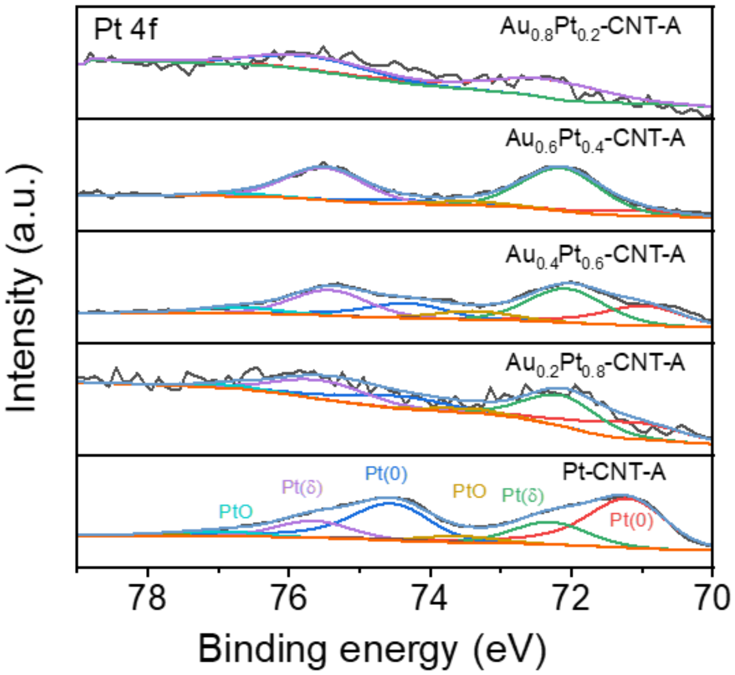


Figure S24. Pt4f spectra of AuPt-CNT-A with different ratio of Au/Pt.

Table S7. XPS measurements of a series of AuPt NCs-CNT-A with different ratio of Au/Pt.

| **Samples** | **Feeding Ratio of Au/Pt** | **Atom ratio Au/Pt** | **Au(0)/Au(I) (%)** | **Pt(0)/Pt(δ) (%)** |
|---|---|---|---|---|
| Au NCs-CNT-A | 1:0 | - | 95.2/4.8 | - |
| $Au_{0.8}Pt_{0.2}$ NCs-CNT-A | 4:1 | 2/1 | 87.7/12.3 | - |
| $Au_{0.6}Pt_{0.4}$ NCs-CNT-A | 3:2 | 1.67/1 | 91.8/8.2 | 7.1/45.9 |
| $Au_{0.4}Pt_{0.6}$ NCs-CNT-A | 2:3 | 1.74/1 | 95.8/4.2 | 19.5/29.5 |
| $Au_{0.2}Pt_{0.8}$ NCs-CNT-A | 1:4 | 0.31/1 | 91.6/8.4 | 24.1/29.7 |
| Pt NCs-CNT-A | 0:1 | - | - | 37.5/14.6 |

Table S8. Comparison of overpotential (η) at current density of -10 mA $cm^{-2}$ with recently reported catalysts in 0.5M $H_2SO_4$ electrolyte.

| Materials | Electrolyte | Overpotential/mV@10 mA $cm^{-2}$ | Reference |
|---|---|---|---|
| $Au_{0.4}Pt_{0.6}$-CNT-A | 0.5 M $H_2SO_4$ | 25 | This work |
| Pt1/NMHCS | 0.5 M $H_2SO_4$ | 40 | [7] |
| Pt–WOx/WS2 | 0.5 M $H_2SO_4$ | 42 | [8] |
| Pt–MoS2 | 0.5 M $H_2SO_4$ | 53 | [9] |
| Pt/C | 0.5 M $H_2SO_4$ | 58 | [10] |
| Pt/np-Co0.85Se | 1.0 M phosphate buffer solutions (PBS, pH =7.0) | 55 | [11] |
| Pt@PCM | 0.5 M $H_2SO_4$ | 105 | [12] |
| Pt-SnS2 | 0.5 M $H_2SO_4$ | 117 | [13] |
| Au–MoS2 | 0.5 M $H_2SO_4$ | 265 | [14] |
| ep-WS2-Pt | 0.5 M $H_2SO_4$ | ~140 | [15] |
| Au33Pt67 | 0.1 M KOH | ~80 | [16] |
| AuPt | 0.5 M $H_2SO_4$ | 250 | [17] |
| Au NF/Pt | 0.5 M $H_2SO_4$ | 100 | [18] |
| Pt1/OLC | 0.5 M $H_2SO_4$ | 38 | [19] |
| Au@NC | 0.5 M $H_2SO_4$ | 130 | [20] |
| d-PdTex | 0.5 M $H_2SO_4$ | 76 | [21] |
| PtSn4 | 0.5 M $H_2SO_4$ | 37 | [22] |

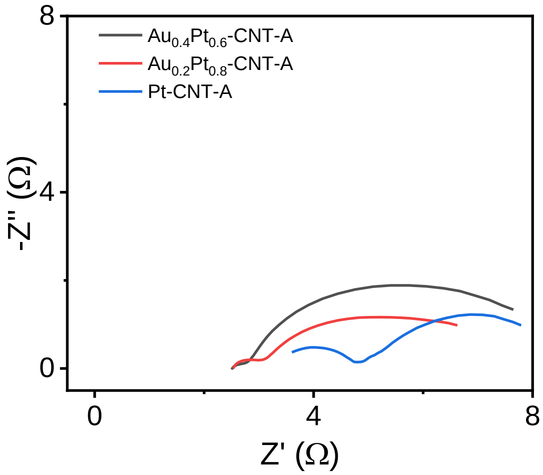


Figure S25. EIS of $Au_{0.4}Pt_{0.6}$-CNT-A.

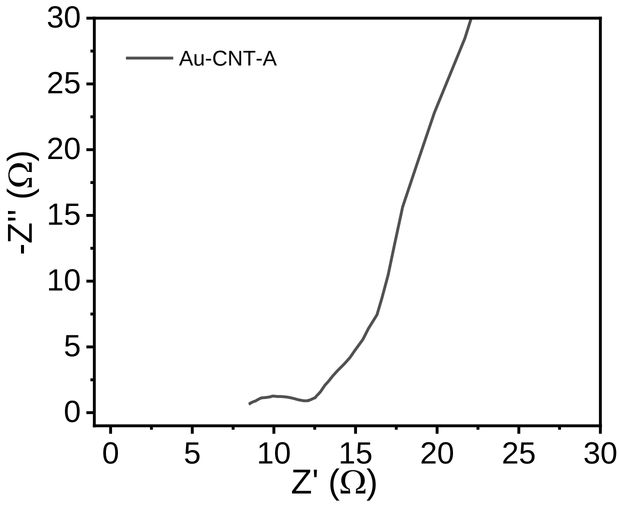


Figure S26. EIS of Au-CNT-A.

Table S9. EIS of $Au_{0.4}Pt_{0.6}$ -CNT-A and compared samples.

| | $R_s$ | $R_{ct}$ |
|---|---|---|
| $Au_{0.4}Pt_{0.6}$-CNT-A | 2.50 | 0.25 |
| $Au_{0.2}Pt_{0.8}$-CNT-A | 2.53 | 0.5 |
| Pt-CNT-A | 3.60 | 1.14 |
| Au-CNT-A | 8.45 | 3.25 |

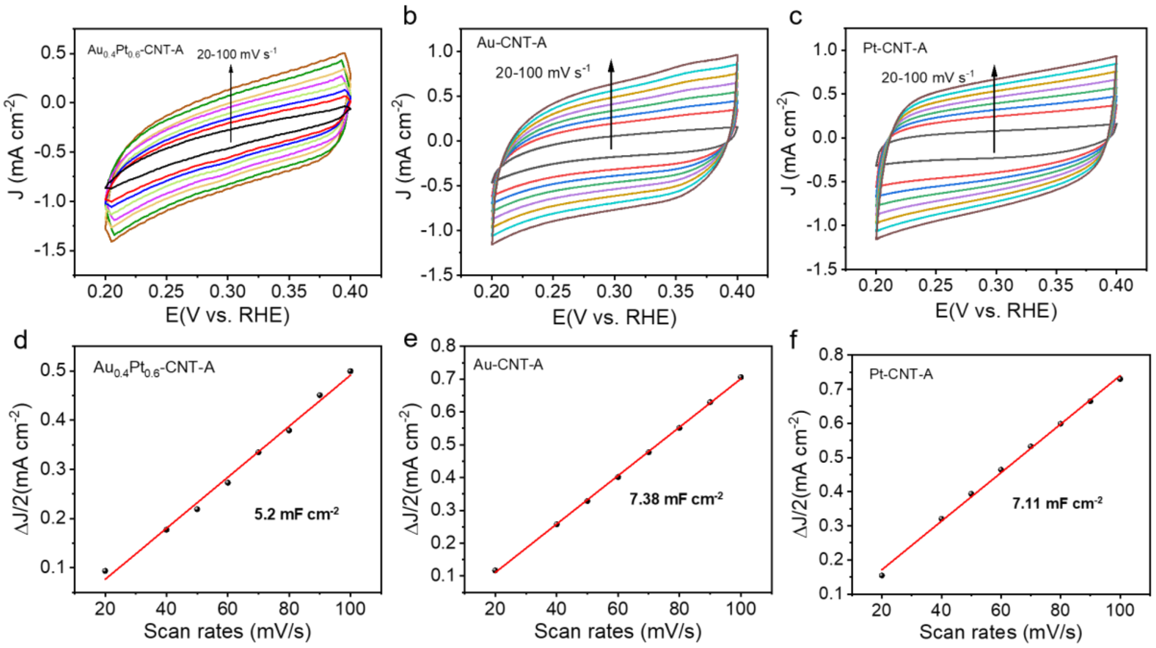


Figure S27. ECSA and $C_{dl}$ of $Au_{0.4}Pt_{0.6}$-CNT-A and referenced samples.

Note that the turnover frequency (TOF) is used to estimate the intrinsic catalytic activity of OER electrocatalysts. The TOF value ($s^{-1}$) is obtained using the following equation:[23,24]

$$TOF = A \times j/(2 \times F \times N) \quad (1)$$

Where $A$ signifies the surface area of the electrode, $j$ indicates the current density at a certain overpotential, $F$ denotes the Faraday constant, and $N$ indicates the number of active sites on the electrode.

Table S10. Comparison of TOF with recently reported catalysts.

| Materials | Electrolyte | Overpotential/mV | TOF($s^{-1}$) | Reference |
|---|---|---|---|---|
| $Au_{0.4}Pt_{0.6}$-CNT-A | 0.5 M $H_2SO_4$ | 100 | 7.63 | Our work |
| Pt–WOx/$WS_2$ | 0.5 M $H_2SO_4$ | 112 | 0.59 | [25] |
| Au-MoS2 | 0.5 M $H_2SO_4$ | 300 | 8.76 | [14] |
| Pt/np-$Co_{0.85}$Se | 1.0 M phosphate buffer solutions (PBS, pH =7.0) | 100 | 3.93 | [11] |
| Pt/C | 0.5 M $H_2SO_4$ | 100 | 1.25 | [26] |
| PtRu/RFCS | 0.5 M $H_2SO_4$ | 100 | 0.375 | [26] |
| Pt@PCM | 0.5 M $H_2SO_4$ | 200 | 10 | [12] |
| Pristine Au NDs | 0.5 M $H_2SO_4$ | 100 | 0.01 | [27] |
| $PtSn_4$ | 1 M KOH | 100 | 1.54 | [22] |
| Pt1/NMHCS | 0.5 M $H_2SO_4$ | 300 | 20.18 | [7] |

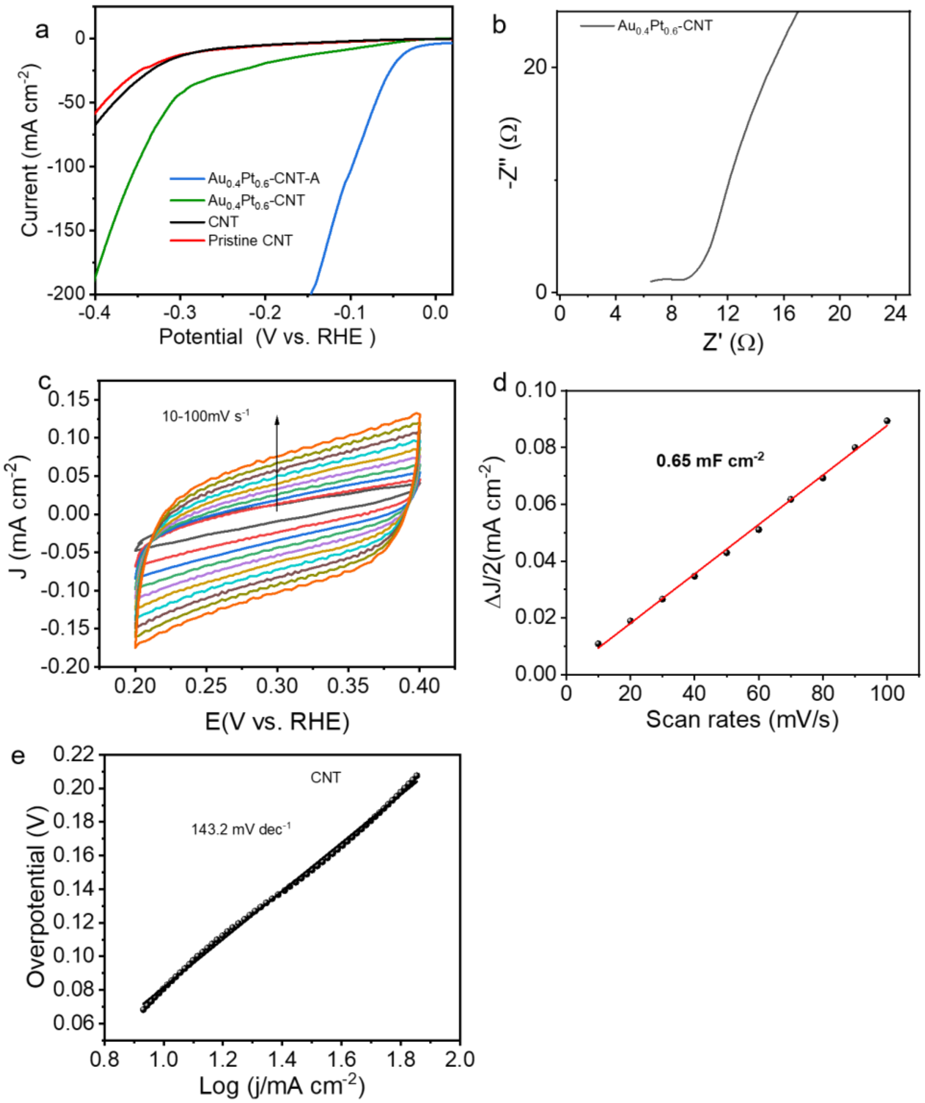


Figure S28. a) LSV, b) EIS, c) ECSA, and d) Cdl of $Au_{0.4}Pt_{0.6}$-CNT and e) Tafel slope of CNT.

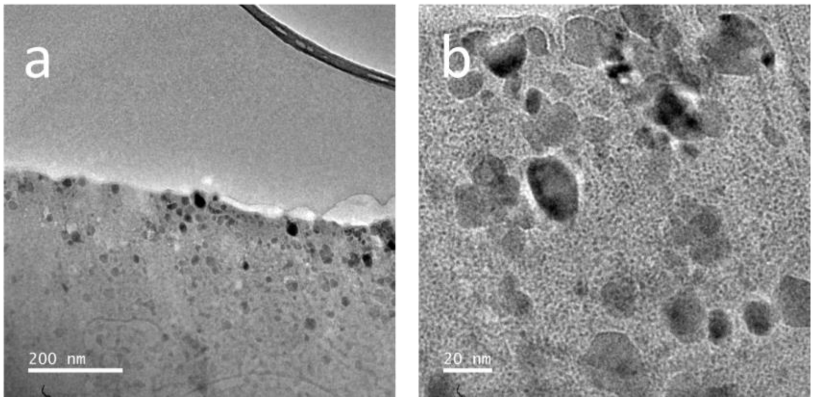


Figure S29. TEM images of $Au_{0.4}Pt_{0.6}$ NCs with annealing without CNT.

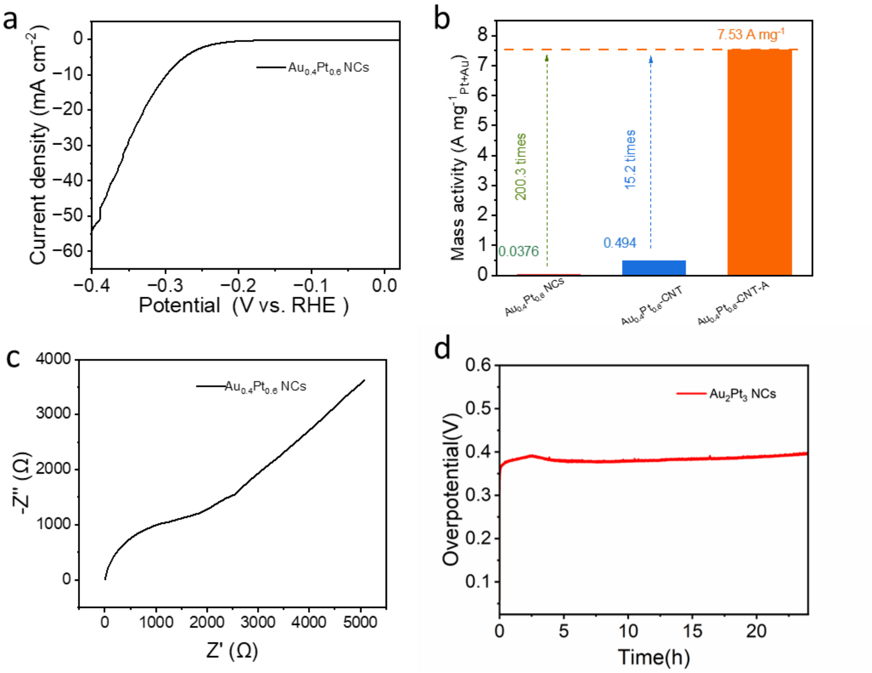


Figure S30. LSV, mass activity, EIS, stability at 10 mA cm$^{-2}$ of $Au_{0.4}Pt_{0.6}$ NCs (2uL (0.34ug at 0.07cm$^2$ GCE electrode).

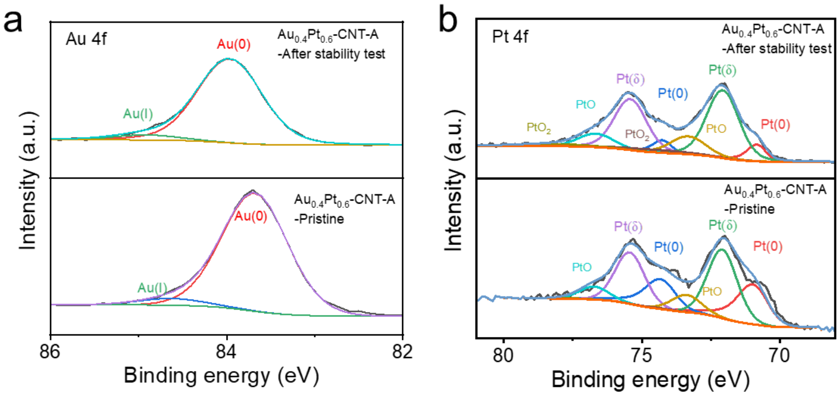


Figure S31. XPS of $Au_2Pt_3$-CNT-A after stability.

# References


1. Ding, E.-X. *et al.* High-performance transparent conducting films of long single-walled carbon nanotubes synthesized from toluene alone. *Nano Res.* **13**, 112–120 (2020).
2. Ding, E.-X. *et al.* Highly conductive and transparent single-walled carbon nanotube thin films from ethanol by floating catalyst chemical vapor deposition. *Nanoscale* **9**, 17601–17609 (2017).
3. Wang, Z.-M. *et al.* Formation of graphite-derived layered mesoporous carbon materials. *Microporous Mesoporous Mater.* **93**, 254–262 (2006).
4. Liu, K. *et al.* Chirality-dependent transport properties of double-walled nanotubes measured in situ on their field-effect transistors. *J. Am. Chem. Soc.* **131**, 62–63 (2009).
5. Luo, Z. *et al.* From Aggregation-Induced Emission of Au(I)–Thiolate Complexes to Ultrabright Au(0)@Au(I)–Thiolate Core–Shell Nanoclusters. *J. Am. Chem. Soc.* **134**, 16662–16670 (2012).
6. Christensen, S. L. *et al.* Dopant location, local structure, and electronic properties of Au24Pt (SR) 18 nanoclusters. *J. Phys. Chem. C* **116**, 26932–26937 (2012).
7. Kuang, P. *et al.* Pt single atoms supported on N-doped mesoporous hollow carbon spheres with enhanced electrocatalytic H2-evolution activity. *Adv. Mater.* **33**, 2008599 (2021).
8. Oh, L. S. *et al.* Unveiling the enhanced electrocatalytic activity at electrochemically synthesized Pt–WO x hybrid nanostructure interfaces. *Chem. Commun.* **57**, 11165–11168 (2021).
9. Huang, X. *et al.* Solution-phase epitaxial growth of noble metal nanostructures on dispersible single-layer molybdenum disulfide nanosheets. *Nat. Commun.* **4**, 1–8 (2013).

10. Sun, L. *et al.* Heterojunction-Based Electron Donators to Stabilize and Activate Ultrafine Pt Nanoparticles for Efficient Hydrogen Atom Dissociation and Gas Evolution. *Angew. Chem. Int. Ed.* **60**, 25766–25770 (2021).

11. Jiang, K. *et al.* Single platinum atoms embedded in nanoporous cobalt selenide as electrocatalyst for accelerating hydrogen evolution reaction. *Nat. Commun.* **10**, 1–9 (2019).

12. Zhang, H. *et al.* Dynamic traction of lattice-confined platinum atoms into mesoporous carbon matrix for hydrogen evolution reaction. *Sci. Adv.* **4**, eaao6657 (2018).

13. Liu, G. *et al.* Efficiently synergistic hydrogen evolution realized by trace amount of Pt-decorated defect-rich SnS2 nanosheets. *ACS Appl. Mater. Interfaces* **9**, 37750–37759 (2017).

14. Shi, Y. *et al.* Hot Electron of Au Nanorods Activates the Electrocatalysis of Hydrogen Evolution on MoS2 Nanosheets. *J. Am. Chem. Soc.* **137**, 7365–7370 (2015).

15. Tang, K., Wang, X., Li, Q. & Yan, C. High Edge Selectivity of In Situ Electrochemical Pt Deposition on Edge-Rich Layered WS2 Nanosheets. *Adv. Mater.* **30**, 1704779 (2018).

16. Wu, W. *et al.* Peptide templated AuPt alloyed nanoparticles as highly efficient bi-functional electrocatalysts for both oxygen reduction reaction and hydrogen evolution reaction. *Electrochimica Acta* **260**, 168–176 (2018).

17. Yu, Y. *et al.* Reconciling of experimental and theoretical insights on the electroactive behavior of C/Ni nanoparticles with AuPt alloys for hydrogen evolution efficiency and Non-enzymatic sensor. *Chem. Eng. J.* **435**, 134790 (2022).

18. Li, M. *et al.* Pt monolayer coating on complex network substrate with high catalytic activity for the hydrogen evolution reaction. *Sci. Adv.* **1**, e1400268 (2015).

19. Liu, D. *et al.* Atomically dispersed platinum supported on curved carbon supports for efficient electrocatalytic hydrogen evolution. *Nat. Energy* **4**, 512–518 (2019).

20. Zhou, W. *et al.* Bioreduction of precious metals by microorganism: efficient gold@ N-doped carbon electrocatalysts for the hydrogen evolution reaction. *Angew. Chem. Int. Ed.* **55**, 8416–8420 (2016).

21. Zuo, Y. *et al.* Defect Engineering in Two-Dimensional Layered PdTe2 for Enhanced Hydrogen Evolution Reaction. *ACS Catal.* **13**, 2601–2609 (2023).

22. Li, G. *et al.* Dirac nodal arc semimetal PtSn4: an ideal platform for understanding surface properties and catalysis for hydrogen evolution. *Angew. Chem.* **131**, 13241–13246 (2019).

23. Yin, J. *et al.* Ni–C–N nanosheets as catalyst for hydrogen evolution reaction. *J. Am. Chem. Soc.* **138**, 14546–14549 (2016).

24. Guo, B. *et al.* 3D Printing of Multiscale Ti64-Based Lattice Electrocatalysts for Robust Oxygen Evolution Reaction. *Adv. Sci.* 2201751 (2022).

25. Xu, J. *et al.* Amorphous MoOX-Stabilized single platinum atoms with ultrahigh mass activity for acidic hydrogen evolution. *Nano Energy* **70**, 104529 (2020).

26. Li, K. *et al.* Enhanced electrocatalytic performance for the hydrogen evolution reaction through surface enrichment of platinum nanoclusters alloying with ruthenium in situ embedded in carbon. *Energy Environ. Sci.* **11**, 1232–1239 (2018).

27. Lai, Y.-H. *et al.* Enhanced hydrogen evolution efficiency achieved by atomically controlled platinum deposited on gold nanodendrites with high-index surfaces. *J. Mater. Chem. A* **9**, 22901–22912 (2021).
